# Supplementary material for: To Perceive or Not to Perceive: Lightweight Stacked Hourglass Network
Source: arXiv:2302.04815 source file (2023-02-09)
Supplement: Supplementary file 1 [file Appendix.tex]

\appendix
\section{Appendix}
\label{sec:appendix}

\subsection{Pooling layers}
\label{app:pooling}
The training loss curve and the validation accuracy curve for different pooling types used are given in Figure. \ref{fig:trainLoss-pool} and \ref{fig:valAcc_pool}. Here, \textit{Base model} refers to the Baseline LeNet-5 which uses Max-pool operation, \textit{Avg pool} refers to the model replacing Max-pool with Average-pool layers, and the \textit{s3p2\_s2} refers to strided convolutions replacing the Max-pool layers where the first convolution uses a $\text{stride}=3$ with $\text{padding}=2$ and the second convolution uses a $\text{stride}=2$.

\begin{figure}[htb]
    \centering
    \includegraphics[width=0.9\columnwidth]{Images/2.1_pooling_trainLoss.png}
    \caption{\centering Training loss with different pooling types}
    \label{fig:trainLoss-pool}
\end{figure}

\begin{figure}[htb]
    \centering
    \includegraphics[width=0.9\columnwidth]{Images/2.1_pooling_valAcc.png}
    \caption{\centering Validation accuracy with different pooling types}
    \label{fig:valAcc_pool}
\end{figure}

\subsection{Dropout}
\label{app:dropout}
In experimenting dropout, dropout before fully connected layers performed best. However, the performance of both 2D and 1D dropouts before the convolution layers gave competitive performance. The performance of different dropout choices is given in Table \ref{tab:dropout_app}. The validation accuracy curve for the best dropout for each setting is given in Figure \ref{fig:dropout}. \par 

\begin{table}[htb]
\caption{Dropout performances}
\label{tab:dropout_app}
\centering
\setcellgapes{2pt}\makegapedcells
\resizebox{\columnwidth}{!}{\begin{tabular}[\columnwidth]{l c c}
    \toprule
    \textbf{Dropout type} & \textbf{Dropout Value} & \textbf{Validation accuracy}\\
    \bottomrule
    \multirow{3}{*}{1D before FC layers} & 0.1 & 65.79\\
    \cline{2-3}\\
    & 0.3 & 61.23\\
    \cline{2-3}\\
    & 0.5 & 60.56\\
    \midrule
    1D before all layers & 0.1 & 64.10\\
    \midrule
    \multirow{3}{*}{1D before CNN layers} & 0.1 & 63.38\\
    \cline{2-3}\\
    & 0.3 & 60.41\\
    \cline{2-3}\\
    & 0.5 & 57.18\\
    \midrule
    \makecell{1D for FC\\ 2D for CNN layers} & 0.1 & 62.76\\
    \bottomrule
\end{tabular}}
\end{table}

\begin{figure}[b]
    \centering
    \includegraphics[width=0.9\columnwidth]{Images/2.2_Dropout_valAcc.png}
    \caption{\centering Validation accuracy with different dropout settings.}
    \label{fig:dropout}
\end{figure}

\subsection{Batch normalization}
\label{app:BN}
Next, we examine the reason behind the improvement in performance when increasing BS to $80$. The statistical estimation that BN performs becomes more accurate as the BS increases since the batch becomes more representative of the distribution of the entire dataset. However, as the BS increases beyond a certain limit, mini-batch SGD becomes more like vanilla gradient descent, which performs sub-optimally for non-convex optimization problems due to local-minima-related reasons. At $BS = 256$, validation accuracy dips to $69.28\%$, as compared to $70.352\%$ when using a BS of $64$. Figure~\ref{fig:trainLoss-bnbs} presents the training loss curves and Figure~\ref{fig:valAcc_bnbs} the validation accuracy curves of the baseline models that include BN layers with different BSs. It can be inferred from Figure~\ref{fig:trainLoss-bnbs} that, as the BS increases, the model's bias increases as well since the weights are being updated based on bigger subsets of the dataset that provide a more general view of the population.

Using momentum with the optimizer, which is akin to the concept of velocity, accelerates convergence by taking into account past updates at each update step (weighted average). The momentum parameter determines the weight of the previous updates in calculating the new update. 

Finally, BN should ideally have a regularization effect on the model. However, We note that for almost all models with BN layers, even though the validation accuracy improved, the gap between the training and validation accuracies was wider as compared to that in the case of the base model with no BN layers. We can not be certain if this is a sign of over-fitting. Assuming it is, we speculate that playing with the momentum parameter of the BN layer, which controls the moving average, might help with that.

\begin{figure}[htb]
    \centering
    \includegraphics[width=\columnwidth]{Images/batch normalization/train-loss-bs.png}
    \caption{\centering Training loss with different batch sizes}
    \label{fig:trainLoss-bnbs}
\end{figure}

\begin{figure}[ht]
    \centering
    \includegraphics[width=\columnwidth]{Images/batch normalization/validation-accuracy-bs.png}
    \caption{\centering Validation accuracy with different batch sizes}
    \label{fig:valAcc_bnbs}
\end{figure}

\subsection{Depthwise separable convolution}
\label{app:depthwiseConv}
Depthwise separable convolutions split the filter into two: a depthwise filter and a pointwise filter. A depthwise operation applies convolution on one channel at a time, preserving the number of channels in the feature map. A pointwise operation applies a convolution filter of size $1 \times 1$ to all channels at a time; the depth of the filter is exactly that of the feature map. The combination of these two operations serves as a replacement to the standard convolution operation, and the number of overall computations is heavily reduced.
